# Supplementary material for: NeuSpell: A Neural Spelling Correction Toolkit
Source: arXiv:2010.11085 source file (2020-10-21)
Supplement: Supplementary file 1 [file appendix.tex]

\section{Appendix}
\label{sec:appendix}

\subsection{Data Collection Sources for \textsc{Word} Strategy}
\label{ssec:sources_word_strategy} 
Sources: \footnote{\href{https://www.dcs.bbk.ac.uk/~ROGER/corpora.html}{https://www.dcs.bbk.ac.uk/}}\textsuperscript{,}\footnote{\href{http://norvig.com/ngrams/spell-errors.txt}{http://norvig.com}}\textsuperscript{,}\footnote{\href{https://en.wikipedia.org/wiki/Wikipedia:Lists_of_common_misspellings/For_machines}{https://en.wikipedia.org/}}\textsuperscript{,}\footnote{\href{http://research.microsoft.com/research/downloads/details/4eb8d4a0-9c4e-4891-8846-7437d9dbd869/details.aspx}{http://research.microsoft.com/research/downloads/}}\textsuperscript{,}\footnote{\href{https://corpus.mml.cam.ac.uk/efcamdat/}{https://corpus.mml.cam.ac.uk/efcamdat/}}\textsuperscript{,}\footnote{\href{https://github.com/facebookresearch/moe}{https://github.com/facebookresearch/moe}}
